# Supplementary material for: "Stones from Other Hills can Polish Jade": Zero-shot Anomaly Image Synthesis via Cross-domain Anomaly Injection
Source: arXiv:2501.15211 source file (2025-03-09)
Supplement: Supplementary file 1 [file X_suppl.tex]

\clearpage
\setcounter{page}{1}
\maketitlesupplementary

\setcounter{figure}{0}
\setcounter{table}{0}

\section{Details of Our New Anomaly Dataset}

Detailed statistics of our new domain-agnostic anomaly dataset are exhibited in Table \ref{tab: Each Anomaly Class Numbers}, which exhibits the specific number of newly-collected real anomalies (OS+RP) and anomalies from existing datasets (ED) in each anomaly class. For real anomalies from existing datasets, we collect 9 publicly-accessible IAD datasets, and categorize their domain-specific anomalies into 8 anomaly classes: AeBAD dataset \cite{zhang2023industrial_sup} records anomalies in the domain of the aero-engine blade, such as holes and stains; DAGM2007 dataset \cite{DAGM2007_sup} collects surface defect images of various textures, such as scratches and stains; MagneticTile dataset \cite{huang2020surface_sup} contains tile images with 6 types of defects, such as abrasions and cracks. MvTec-AD dataset \cite{bergmann2019mvtec_sup} contains images from 15 categories, which include rich anomaly patterns like cracks, scratches and holes. MvTec-LOCO-AD dataset \cite{bergmann2021mvtecloco_sup} includes 5 object categories with structural anomalies, such as scratches, pits, or stains, while logical anomalies in this dataset are not included as we do not discuss the synthesis of logical anomalies in this paper. RSDDs dataset \cite{zhang2018railway_sup} records the rail surface defects (mainly orifices and stains) from the actual scenes, and its images contain complex backgrounds and noise. VisA dataset \cite{zou2022spot_sup} contains 12 commonly-seen objects from different domains, while it includes anomalies like scratches, pits, cracks, and stains. VTADL dataset \cite{mishra2021vt_sup} captures anomaly images from 3 types of industrial products that contain abrasions and stains. CrackForest dataset \cite{shi2016automatic_sup} collects images of road cracks. Apart from the existing IAD dataset above, one can certainly extend our cross-domain anomaly dataset by introducing real anomalies from any other IAD dataset. \\

\section{Details of CAI-guided Diffusion Model}

Specifically, for anomaly class $\mathcal{C}_j$ in a specific domain, CAI synthesizes $N'$ pseudo anomaly images of anomaly class $\mathcal{C}_j$: $\mathcal{I}_j^{(sa)}=\{I_i^{(sa)}\}^{N'}_{i=1}$, which are used as training data to guide anomaly generation. LDM is used as the generative model. To extract common anomaly features of $\mathcal{C}_j$, CDM uses Textual Inversion (TI) \cite{DBLP:conf/iclr/GalAAPBCC23}, which can learn those features by an embedding $e$ with very few samples (e.g. 3-5). The learned $e$ then serves as the condition that guides LDM to generate more pseudo anomalies of $\mathcal{C}_j$. To facilitate learning anomaly appearance and location separately, CDM follows \cite{hu2024anomalydiffusion} to decouple $e$ into an anomaly embedding $e_a$ and a spatial embedding $e_s$: $e=\{e_a, e_s\}$. To incorporate prior knowledge of anomalies into training, $e_a$ and $e_s$ are initialized as follows: For $e_a$, it is initialized by the word embeddings of a textual description about $I_i^{(sa)}$'s domain and anomaly class, e.g. ``\texttt{A photo of a capsule+crack}''. As to $e_s$, we first build a location mask $y_i^{(loc)}$ to indicate the core location of injected anomaly pattern in the pseudo anomaly image $I_i^{(sa)}$:

\begin{equation}
    y_i^{(loc)}(l)=\left\{
\begin{aligned}
1, & \qquad  l\in \Omega(I^{(n)}, l_c, A') \\
0, & \qquad  otherwise. 
\end{aligned}
\right.
\end{equation}
where $I^{(n)}, l_c$ and $ A'$ denote the target image, injection location and injected anomaly pattern of $I_i^{(sa)}$, while $\Omega(I^{(n)}, l_c, A')$ refers to the region that $A'$ occupies when it is centered at $l_c$ of $I^{(n)}$. Note that we use $y_i^{(loc)}$ rather than $y^{(sa)}$ in Eq. (\ref{eq:mask}), so as to focus on the core anomaly pattern and ignore less important pixel changes caused by PE. Then, $y_i^{(loc)}$ is encoded into $e_s$ by a an spatial encoder $E_s$ (detailed in supplementary material). With initialized $e=\{e_a, e_s\}$, we train a LDM $G_a$ to learn $e$ and $E_s$ \cite{DBLP:conf/iclr/GalAAPBCC23}:

\begin{equation}
    \begin{aligned}
      e^*, E^*_s = & \arg\min_{e, E_s}\mathbb{E}_{z_i\sim E_a(I_i^{(sa)}), y_i^{(loc)},\epsilon, t}\mathcal{L}_{TI}, \\
      \mathcal{L}_{TI} = & ||y_i^{(loc)}\odot (\epsilon - \epsilon_\theta(z_i^t, t, e))||^2_2
    \end{aligned}
\end{equation}
where $E_a$ is the image encoder of $G_a$ that encodes $I_i^{(sa)}$ into a latent code $z_i$, $\epsilon\sim \mathcal{N}(0, 1)$ is a Gaussian noise and  $\epsilon_\theta$ denotes the noise estimated by $G_a$ parameterized by $\theta$ at time step $t$. Pixel-wise multiplication with $y_i^{(loc)}$ aims to make the model focus on learning the anomaly patterns in the injected region \cite{hu2024anomalydiffusion}.  Meanwhile, another LDM $G_m$ is trained as an anomaly mask generator $G_m$ by $y_i^{(loc)}$ and TI, which generates diverse anomaly masks to appoint the locations of generated pseudo anomalies. As to anomaly generation, $G_m$ first generates a new mask $y^{(g)}$ and then encodes it into $e^{(g)}_s$ by the trained spatial encoder $E_s$. Then, we fetch $e_a$ from the learned $e^*$ to denote anomaly appearance, and a condition embedding $e'$ is yielded by $e'=\{e_a, e^{(g)}_s\}$. Finally, a new pseudo anomaly image can be generated by feeding $e'$ and a target normal image $I^{(n)}{}'$ into $G_a$. Besides, we leverage Adaptive Attention Re-weighting \cite{hu2024anomalydiffusion} and blended diffusion process \cite{avrahami2022blended} to ensure a fulfilled and smooth generation. 

For our CDM, its anomaly generator $G_a$ and mask generator $G_m$ adopt the LDM architecture\footnote{https://ommer-lab.com/files/latent-diffusion/nitro/txt2img-f8-large/model.ckpt} of Stable Diffusion \cite{rombach2022high}. As to the spatial encoder $E_s$, we use the network architecture from the FSAS solution ADiff \cite{hu2024anomalydiffusion}: A pre-trained ResNet-50 network \cite{he2016deep} is used as backbone to extract features from input mask images, while features from multiple layers of the backbone are fed into a Feature Pyramid Network \cite{lin2017feature} to obtain the fused feature. Then, several fully-connected networks are introduced to convert the fused feature into tokens of the spatial embedding $e_s$. The token number of anomaly embedding $e_a$, spatial embedding $e_s$ and mask embedding are set to 8, 4 and 4, respectively. 

As to the training of CDM, we synthesize 5 representative pseudo anomaly images by CAI for each anomaly class as training data of CDM. We then adopt a similar training process to \cite{hu2024anomalydiffusion}: Data augmentations (random cropping, rotation and translation) are performed on the pseudo images and their location masks to enhance generation. In order to keep the anomaly pattern within the image during data augmentation, we constrain the augmentation by recoding the maximum/minimum coordinates of the anomaly pattern. Then, the training of CDM is conducted as follows: First, we train the LDM $G_a$ and spatial encoder $E_s$ for 300000 epochs with all pseudo anomalies. Then, we train the anomaly mask generator $G_m$ by 30000 epochs for each anomaly class. Meanwhile, we use a batch size of 4 and a learning rate of 0.005 when training both $G_a$ and $G_m$. The Adam optimizer \cite{kingma2014adam} is utilized in the training process.
\begin{figure*}[t]
  \centering
   \includegraphics[width=1\linewidth]{figure/sup_all.pdf} 
   \caption{8 classes of pseudo anomaly images synthesized by CAI, using target images from different datasets.}
   \label{fig:sup_all}
\end{figure*}
%Figure \ref{fig: CAI_bottle_for_CDM}, \ref{fig: CAI_leather_for_CDM}  shows that the anomalies generated by CDM are similar but not the same as those generated by CAI. The top 5 are whole training data for CDM, then generated a large number of anomalies.

% resnet-based \cite{he2016deep} feature extractor to obtain multi-level features, then fuse them to fully connected networks, which exports the final spatial embedding. After obtaining the trained  $e_a$ and mask embedding, we input them to stable diffusion to obtain the required pseudo anomalies and masks.

% [We also trained the CDM on the VisA dataset] 

\begin{table}[t]
\caption{Statistics of our new domain-agnostic anomaly dataset. ``OS+RP'' refers to the number of newly-collected real anomaly data from online search and reality photographing, while ``ED'' refers to the number of real anomalies from existing datasets.}
\centering
\resizebox{0.3\textwidth}{!}{ % 调整表格大小，宽度为文本宽度的70%
\begin{tabular}{l|cccc}
\toprule[0.5pt]
 & OS+RP & ED & Class number \\
\midrule
Pits & 199 & 362 & 561 \\
Hole & 201 & 896 & 1097 \\
Stain & 164 & 940 & 1104 \\  
Crack & 221 & 631 & 852 \\  
Orifice	& 164 & 33 & 197 \\
Scratch	& 180 & 872 & 1052 \\
Abrasion & 137 & 536 & 673 \\
Impurity & 101 & 301 & 402 \\
\midrule
Total & 1367 & 4571 & 5938 \\
\bottomrule[0.5pt]
\end{tabular}}
\label{tab: Each Anomaly Class Numbers}
\end{table}

\section{Details of Implementation and Evaluation}

\begin{figure*}[h]
  \centering
   \includegraphics[width=0.8\linewidth]{figure/sup_all_CDM.pdf} 
   \caption{Pseudo anomaly images generated by CDM on different datasets.}
   \label{fig:sup_all_CDM}
\end{figure*}

\subsection{Competing ZSAS Methods}
% Describe the settings of competing baselines. Describe the way to obtain training data, and the detailed architecture of the UNet detector we use. 
In this section, we first elaborate on the implementation details of SOTA ZSAS solutions that are used for comparison. We notice that existing ZSAS solutions are typically accompanied by other modules or boosting tricks to perform IAD. To concentrate on ZSAS alone, we extract their ZSAS component and retain their original settings, while their synthesized pseudo anomalies are fed into our unified IAD framework for evaluation. Implementation details of each competing ZSAS solution are provided as follows:  
%data preparation module in the model training pipeline. After data augmentation, the prepared data is directly fed into the model training process, and these methods often lack independent code for generating pseudo-anomalies. Consequently, we have retained the original settings from the source code and extracted the image generation component to serve as baseline experiments in all fairness. The relevant code will be released Upon acceptance to facilitate further research in the field of ZSAS.
\textbf{CutPaste} \cite{li2021cutpaste} is the pioneering model-free ZSAS solution. As no official implementation is provided, we adopt the re-implementation from a popular PyTorch project\footnote{https://github.com/Runinho/pytorch-cutpaste}. CutPaste offers four operational modes: CutPasteNormal, CutPasteScar, CutPasteUnion and CutPaste3Way. In this paper, we select the CutPaste3Way mode as it demonstrates superior performance when compared with other modes \cite{li2021cutpaste}. \textbf{NSA} \cite{schluter2022natural} is a model-free solution that is developed based on CutPaste, and we adopt the official implementation of NSA\footnote{https://github.com/hmsch/natural-synthetic-anomalies}. NSA also leverages Poisson Editing to inject normal image patches, and we set the mode of PE to be \textit{Normal} for both NSA and our CAI, as it often yields slightly better performance. \textbf{DRAEM} \cite{zavrtanik2021draem} is a widely-used model-free ZSAS solution, which is retrieved from the official repository of DRAEM\footnote{https://github.com/VitjanZ/DRAEM}. \textbf{GLASS} \cite{chen2024unified} is the latest model-free ZSAS solution that is based on DRAEM, and it is adopted from its official implementation\footnote{https://github.com/cqylunlun/GLASS} for our experiments. \textbf{RealNet} \cite{zhang2024realnet} is the latest model-based ZSAS solution, while we extract its ZSAS module from the official implementation\footnote{https://github.com/cnulab/RealNet} for our evaluation and comparison. Apart from the above ZSAS solutions, we also include a SOTA model-based FSAS solution, \textbf{ADiff} \cite{hu2024anomalydiffusion}, as a reference, while we directly use its official implementation\footnote{{https://github.com/sjtuplayer/anomalydiffusion}}. It is worth noting that ADiff actually uses one-third of domain-specific anomalies in the test set as training data, which renders it a strong competitor. 

%enhances DRAEM by incorporating double-Perlin noise and employing intersection or union operations to produce a greater diversity of pseudo anomalies. Additionally, it utilizes a matting strategy to effectively filter out anomalies that lie outside the foreground. We meticulously followed its design principles and generated ten anomalous images for each normal image.

% The anomalies texture sources are generated by introducing disturbances during the reverse recovery phase of the diffusion model. These anomaly textures, derived from diffusion, are then integrated into the target normal image using a Perlin noise technique similar to that employed in DRAEM, resulting in artificial anomalies that lack authenticity in their visual representation.

\subsection{Details of Evaluation}
\begin{table*}[t]
 % 调整行间距
\setlength\tabcolsep{2pt} % 减少列间距
\small % 使用较小字体
\caption{Detailed pixel-level performance (AUC/AP/PRO, \%) on MvTec-AD dataset.}
\centering
\begin{tabular}{l|cccccccc}
\toprule
~ & CutPaste & NSA-N & NSA-M & DRAEM & RealNet & GLASS & CAI-N & CAI-M  \\
\midrule
Bottle & 85.3/35.9/64.4 & 98.0/82.1/90.4 & 94.9/63.9/80.9 & 86.5/56.1/71.8 & 85.7/54.7/67.4 & 92.2/67.7/80.5 & 97.3/73.7/87.0 & 96.1/67.6/83.7  \\
Capsule & 87.2/7.2/73.8 & 89.9/35.7/77.3 & 86.9/23.9/54.9 & 83.6/17.5/73.2 & 94.7/30.8/90.5 & 88.4/22.3/74.9 & 95.7/47.1/89.8 & 94.6/46.5/88.6  \\
Carpet & 95.3/49.0/79.6 & 92.8/48.3/73.3 & 98.7/78.3/94.3 & 96.2/67.5/90.6 & 89.2/39.9/70.3 & 95.2/62.2/88.1 & 98.5/75.0/94.2 & 98.4/73.0/93.6  \\
Leather & 96.9/59.8/94.2 & 94.6/42.4/91.8 & 99.6/67.6/98.2 & 98.3/70.1/96.6 & 97.5/57.0/94.7 & 95.0/54.2/90.9 & 99.4/70.0/97.8 & 99.4/70.4/97.8  \\
Pill & 90.6/52.8/61.1 & 94.9/64.8/78.9 & 95.9/64.1/84.1 & 92.4/55.7/87.8 & 97.3/80.8/80.1 & 97.4/79.1/91.7 & 97.5/73.8/91.9 & 98.0/79.1/94.1  \\
Transistor & 69.9/18.7/51.5 & 73.2/28.6/53.0 & 65.3/19.9/44.7 & 67.4/24.3/52.4 & 64.4/17.5/53.9 & 66.6/20.0/52.4 & 76.8/32.6/62.3 & 70.3/29.8/59.2  \\
Tile & 92.2/39.7/77.7 & 95.4/75.5/89.1 & 95.9/79.6/91.0 & 98.9/94.2/96.4 & 91.8/73.3/82.4 & 98.4/91.0/94.5 & 99.0/89.9/95.9 & 98.6/85.6/95.9  \\
Cable & 79.5/12.4/52.6 & 87.5/24.6/80.6 & 85.6/14.1/67.9 & 81.3/28.4/60.9 & 74.6/5.8/36.5 & 82.8/10.9/60.5 & 93.8/52.3/78.2 & 89.2/51.7/72.0  \\ 
Zipper & 95.6/53.2/83.7 & 97.1/76.3/91.3 & 98.8/80.5/95.1 & 96.9/68.4/87.9 & 83.8/35.1/61.1 & 95.2/62.1/83.8 & 93.8/63.6/82.3 & 92.2/59.2/77.7  \\
Toothbrush & 88.5/17.3/57.9 & 91.2/18.5/66.7 & 85.5/21.1/63.2 & 90.5/40.6/77.5 & 86.6/21.2/68.6 & 92.6/42.5/81.1 & 95.1/40.3/82.6 & 96.1/34.8/83.2  \\
Metal\_nut & 87.4/50.9/51.4 & 96.5/85.7/82.3 & 83.1/39.5/62.3 & 90.4/63.4/85.6 & 68.8/20.9/58.5 & 82.2/52.7/80.3 & 98.6/91.7/89.6 & 98.4/91.1/88.5  \\
Hazelnut & 98.0/72.2/93.9 & 97.8/50.6/92.2 & 98.3/56.5/93.1 & 97.4/68.5/96.1 & 88.8/50.8/89.4 & 96.8/67.2/96.0 & 98.8/75.7/93.1 & 98.8/75.7/94.1  \\
Screw & 90.0/9.5/69.3 & 92.2/15.1/73.6 & 93.9/18.9/81.0 & 93.6/30.0/82.2 & 96.8/32.0/86.6 & 95.0/51.2/88.5 & 95.8/31.6/84.0 & 96.5/35.8/86.5  \\
Grid & 90.8/21.0/78.4 & 98.5/50.2/95.6 & 96.0/38.8/91.8 & 95.9/56.3/90.5 & 68.8/6.2/46.2 & 93.2/68.8/86.1 & 96.7/44.1/91.4 & 97.2/46.9/92.2  \\
Wood & 96.4/77.5/88.9 & 85.7/37.6/72.6 & 89.4/42.0/79.1 & 95.4/76.4/88.4 & 87.1/58.7/77.8 & 95.8/28.6/85.0 & 97.3/77.3/92.1 & 97.3/77.2/91.6  \\
\midrule
Aevrage & 89.6/38.5/71.9 & 92.4/49.1/80.6 & 91.2/47.2/78.8 & 91.0/54.5/82.5 & 85.1/39.0/70.9 & 91.1/52.0/82.3 & \textbf{95.6/62.6/87.5} & \ul{94.7}/\ul{61.6}/\ul{86.6}  \\ \hline 
\bottomrule[0.75pt]
\end{tabular}
\label{tab: MvTec-AD pixel AUC/AP/PRO}
\end{table*}

\begin{table*}[t]
 % 调整行间距
\setlength\tabcolsep{2pt} % 减少列间距
\small % 使用较小字体
\caption{Detailed pixel-level performance (AUC/AP/PRO, \%) on VisA dataset.}
\centering
\begin{tabular}{l|ccccccccc}
\toprule
~ & CutPaste & NSA-N & NSA-M & DRAEM & RealNet & GLASS & CAI-N & CAI-M  \\ 
\midrule
Candle & 87.8/7.7/69.2 & 97.3/39.5/85.5 & 97.9/38.3/88.7 & 90.7/34.8/90.6 & 89.9/24.7/90.5 & 89.4/28.8/91.0 & 94.6/32.0/88.9 & 94.7/33.8/89.8  \\
Capsules & 92.9/16.9/58.1 & 98.0/58.8/79.0 & 98.7/51.9/88.3 & 92.0/31.9/88.0 & 83.2/1.8/55.5 & 90.4/15.3/71.5 & 98.6/59.6/93.3 & 98.0/56.0/91.8  \\
Cashew & 91.0/7.3/60.7 & 93.4/17.8/91.4 & 93.1/15.5/90.2 & 93.3/29.4/86.5 & 92.9/12.4/86.5 & 92.6/15.3/72.6 & 95.8/40.5/93.8 & 95.9/39.0/94.0  \\
Chewinggum & 94.4/32.3/68.9 & 98.8/74.6/81.6 & 99.2/56.2/86.4 & 98.5/64.7/87.0 & 99.1/84.6/92.2 & 98.4/48.6/82.8 & 98.7/45.9/80.9 & 98.5/56.8/82.4  \\
Fryum & 92.7/27.2/83.3 & 95.2/43.4/80.0 & 92.6/30.5/78.4 & 94.9/50.4/84.0 & 94.3/31.2/89.4 & 93.8/31.3/83.1 & 96.0/54.2/86.1 & 96.7/55.6/89.5  \\
Macaroni1 & 96.4/2.5/81.9 & 99.5/40.3/95.2 & 99.2/32.1/92.9 & 99.1/52.5/91.6 & 99.8/37.9/95.2 & 99.1/40.3/92.0 & 99.9/44.5/96.9 & 99.9/42.7/97.2  \\
Macaroni2 & 95.5/3.4/83.1 & 95.5/2.7/83.8 & 94.1/2.8/83.5 & 96.5/21.8/90.2 & 98.2/10.2/93.1 & 98.3/20.7/92.6 & 98.8/23.0/92.4 & 99.4/25.8/93.3  \\
Pcb1 & 92.8/34.5/52.2 & 95.0/59.2/69.8 & 91.6/10.9/67.2 & 93.2/53.1/70.3 & 35.5/0.9/43.3 & 83.4/20.0/40.4 & 98.2/64.3/78.4 & 97.9/47.8/83.0  \\
Pcb2 & 90.9/10.2/64.0 & 95.6/29.7/85.2 & 92.2/18.3/74.3 & 86.9/21.8/74.3 & 72.0/1.1/46.1 & 83.2/13.0/60.8 & 93.6/27.3/80.5 & 94.7/29.8/81.0  \\
Pcb3 & 93.6/2.5/79.5 & 87.5/6.0/86.0 & 85.8/1.6/79.1 & 83.6/11.1/86.1 & 77.5/9.3/85.3 & 79.3/10.3/84.6 & 88.5/5.6/86.2 & 84.9/5.2/86.9  \\
Pcb4 & 93.1/16.6/77.8 & 95.0/22.5/78.9 & 91.3/9.8/76.4 & 91.8/26.8/84.1 & 88.4/26.4/77.7 & 90.7/27.8/84.0 & 91.6/15.7/79.5 & 92.0/20.9/83.8  \\
Pipe-fryum & 95.1/28.7/87.2 & 97.6/52.7/90.3 & 97.7/42.8/95.2 & 97.5/48.8/94.3 & 95.2/21.7/94.1 & 97.9/52.5/94.2 & 98.7/63.6/95.3 & 98.7/68.1/96.2  \\
\midrule
Average & 93.0/15.8/72.2 & 95.7/37.3/83.9 & 94.5/25.9/83.4 & 93.2/37.3/85.6 & 85.5/21.8/79.1 & 91.4/27.0/79.1 & \textbf{96.1}/\ul{39.7}/\ul{87.7} & \ul{95.9}/\textbf{40.1}/\textbf{89.1}  \\
\bottomrule[0.75pt]
\end{tabular}
\label{tab: VisA pixel AUC/AP/PRO}
\end{table*}

As to evaluation, our unified IAD framework is designed based on \cite{hu2024anomalydiffusion}, which is the latest work that conducts a specialized discussion and comparison on anomaly synthesis: The IAD is carried out by a UNet \cite{ronneberger2015u} model that adopts the encoder-decoder architecture from \cite{zavrtanik2021draem}. The encoder is composed of six convolutional blocks and five max-pooling layers. Each convolutional block consists of two 3$\times$3 convolutional layers with padding 1, followed by a batch normalization and ReLU activation layer. The decoder is composed of four 2$\times$ upsampling layers, four double convolutional blocks and a final 3$\times$3 convolutional layer. To prevent performance saturation that weakens the performance difference of different ZSAS solutions, we deliberately avoid using any additional modules or boosting tricks. For each target image from the normal train set, we synthesize ten pseudo anomalies and construct a pseudo anomaly set. To further reduce performance saturation and promote computational efficiency, We randomly select 1000 images of the pseudo anomaly set as the training data for all ZSAS solutions. Then, the UNet is trained by the default Focal loss of the PyTorch framework\footnote{{https://pytorch.org/}}, while we use a batch size of 8, a learning rate of 0.0001 and the Adam optimizer. The random seed is fixed to 42. The evaluation is carried out in a programming environment with Python 3.8 and PyTorch 2.3.1, which is based on a workstation with 128 GiB RAM, NVIDIA A6000 GPU and Intel Xeon 5218R CPU.

% \begin{figure}[t]
%   \centering
%    \includegraphics[width=1.\linewidth]{figure/sup_figure_1.pdf} 
%    \caption{Selected 5 CAI-based leather abrasion images and generated 15 CDM-based images  }
%    \label{fig:CAI_bottle_for_CDM}
% \end{figure}

% \begin{figure}[t]
%   \centering
%    \includegraphics[width=1.\linewidth]{figure/sup_figure_2.pdf} 
%    \caption{Selected 5 CAI-based bottle hole images and generated 15 CDM-based images  }
%    \label{fig:CAI_leather_for_CDM}
% \end{figure}
\subsection{Detailed Experimental Results}

Since MvTec-AD and VisA contain multiple subsets, we first exhibit the detailed performance of ZSAS solutions on each subset in Table \ref{tab: MvTec-AD pixel AUC/AP/PRO}-\ref{tab: VisA pixel AUC/AP/PRO}. Second, we also present a more extensive exhibition of pseudo anomalies synthesized by CAI in Fig. \ref{fig:sup_all}, which demonstrates CAI's capability in synthesizing diverse and authentic pseudo anomalies in various domains. Third, we show more pseudo anomaly images generated by the proposed CDM in Fig. \ref{fig:sup_all_CDM}, so as to further demonstrate its ability in extending pseudo anomalies. 

\subsection{Additional Remarks}

\begin{table}[t]
\small
\caption{Computational cost of model-free baselines}
\centering
\resizebox{0.35\textwidth}{!}{ % 调整表格大小，宽度为文本宽度的70%
\begin{tabular}{l|cccc}
\toprule[0.5pt]
 & Time (s) per image \\
\midrule
CutPaste &  0.013\\
NSA-N & 0.007\\
NSA-M & 0.007\\
DRAEM & 0.011\\  
GLASS & 0.009\\
RealNet (only inference) &  0.026\\
CAI-N & 0.019\\
CAI-M & 0.018\\
\bottomrule[0.5pt]
\end{tabular}}
\label{tab: Computational cost}
\end{table}

We would also like to make the following remarks:  (1) \textit{Number of synthesized pseudo anomalies.} We also vary the number of synthesized pseudo anomalies in \textit{Normal} mode, and test their influence on CAI's performance: Apart from the case where 10 images are synthesized (CAI-10), we also test the case where 5 and 20 pseudo anomalies are synthesized (CAI-5 and CAI-20) for our evaluation. As shown in Fig. \ref{fig:cai_5_10_20}, the influence of pseudo anomaly number on performance is actually minor, and increasing the number of pseudo anomalies does not necessarily improve performance. Thus, we simply select 10 by default to evaluate ZSAS. (2) \textit{Computational cost.} we present the average computation time of different methods to synthesize one pseudo anomaly image on the MvTec-AD dataset, which is shown in Table \ref{tab: Computational cost}. All compared methods are executed in parallel on 40 cores except for RealNet, which is excuted on 80 cores due to its large computational overhead. Besides, for RealNet, the reported computational cost does not contain the cost of training the diffusion model, which is actually the major bottleneck. As shown by Table \ref{tab: Computational cost}, the computational cost of cAI is fairly acceptable, since it takes less than 0.02 second to synthesize one anomaly image. Meanwhile, apart from RealNet, CAI takes slightly more time than other methods due to the following  reasons: First, CAI requires Poisson editing over a more irregular and larger area, which accounts for the major part of computational cost; Second, CAI involves frequent reading of real anomaly image files from the DAAD dataset, introducing additional time consumption; Third, the proposed STM and multi-scale anomaly synthesis also incur computational burden. Finally, it is important to note that the synthesis of pseudo anomalies does not influence the deployment of the IAD model. These images can be fully synthesized offline before participating in the training and inference process.

\begin{figure}[t]
  \centering
   \includegraphics[width=0.6\linewidth]{figure/sup_figure_3.pdf} 
   \caption{Different numbers of synthesized pseudo anomalies.}
   \label{fig:cai_5_10_20}
\end{figure}

\bibliography{main}
